# Supplementary material for: Haldane Quantum Hall Effect for Light in a Dynamically Modulated Array of Resonators
Source: arXiv:1507.04541 source file (2015-10-09)
Supplement: Supplementary file 1 [file dynamic_supplementary.pdf]

# Supplemental Material for: Haldane Quantum Hall Effect for Light in a Dynamically Modulated Array of Resonators

Momchil Minkov* and Vincenzo Savona
*Laboratory of Theoretical Physics of Nanosystems,*
*Ecole Polytechnique Fédérale de Lausanne (EPFL), CH-1015 Lausanne, Switzerland*
(Dated: October 7, 2015)

### Floquet theory

We start from the most general, linear, time-independent Hamiltonian for photons on a lattice ($\hbar = 1$):

$$H_S = H_0 + H_J = \sum_i \omega_i a_i^\dagger a_i - \sum_{i \neq j} J_{ij} a_i^\dagger a_j, \tag{1}$$

with $a_i^\dagger$, the photon creation operator, and no particular requirements for the couplings $J_{ij}$ (these will come later depending on the chosen lattice geometry). We add an on-site, time-dependent, periodic modulation of the resonant frequency with a position-dependent intensity and phase

$$H_t = \sum_i A_i \cos(\Omega t + \phi_i) a_i^\dagger a_i. \tag{2}$$

For times much larger than the period $T = 2\pi/\Omega$, it becomes meaningful to apply the Floquet theory of quasi-energies [1, 2]. In particular, the solutions to the time-dependent Schrödinger equation can be written as $|\psi_n(t)\rangle = \exp(-i\varepsilon_n t)|u_n(t)\rangle$, with $u_n(t)$ a $T$-periodic function which is a solution to

$$[H_S + H_t - i\partial_t]|u_n(t)\rangle = \varepsilon_n |u_n(t)\rangle \tag{3}$$

The spectrum $\varepsilon_n$ has a Brillouin-zone like structure with $\Omega$ the width of the first zone, i.e. for any solution $|u_n(t)\rangle$ of quasi-energy $\varepsilon_n$, and any integer $m$, $\exp(im\Omega t)|u_n(t)\rangle$ is also a solution, with eigenvalue $\varepsilon_n + m\Omega$. The states $|u_n(t)\rangle$ form a Hilbert space of $T$-periodic functions. The inner product in this space can be defined starting from the standard bra-ket inner product $\langle \bullet | \bullet \rangle$ for time-independent states, and reads

$$\langle\langle \bullet | \bullet \rangle\rangle T \int_0^T \mathrm{d}t \langle \bullet | \bullet \rangle, \tag{4}$$

The states can be expanded on the Floquet basis given by

$$\begin{aligned} |\{n_i\}, m\rangle &= U_t(t)|\{n_i\}\rangle \exp(im\Omega t) \qquad (5)\\ &= |\{n_i\}\rangle \exp\left(-\frac{i}{\Omega}\sum_i A_i \sin(\Omega t + \phi_i) n_i + im\Omega t\right), \end{aligned}$$

where $n_i$ denotes the occupation number of site $i$, and

$$U_t(t) = \exp\left(-i\int_{t_0}^t H_t(t')\mathrm{d}t'\right) \tag{6}$$

is the time-evolution operator corresponding to the time-dependent Hamiltonian $H_t$, and we assume an adiabatic switching of the modulation in order to disregard the phase offset due to the starting time $t_0$. Since the Hamiltonian is particle-number-preserving, we need only consider the subspace of a single excitation in the system, $\sum_i n_i = 1 \; \forall \; \{n_i\}$. Equation (3) is then an eigenvalue problem with matrix elements in this basis given by

$$\begin{aligned} &\langle\langle \{n'_j\}, m'|H_S + H_t - i\partial_t|\{n_i\}, m\rangle\rangle = \qquad (7)\\ &\delta_{m,m'}\left[\langle \{n'_j\}|H_0 + m\Omega|\{n_i\}\rangle\right] + \\ &\int_0^T e^{i(m-m')\Omega t} \exp\left(\frac{iA_j}{\Omega}\sin(\Omega t + \phi_j) - \frac{iA_i}{\Omega}\sin(\Omega t + \phi_i)\right) \\ &\times \langle \{n_j\}|H_J|\{n_i\}\rangle. \end{aligned}$$

These matrix elements are then equal to

$$\langle\langle n'_i, m'|H_S + H_t - i\partial_t|n_i, m\rangle\rangle = \delta_{m,m'}\left(m\Omega + \omega_i\right), \tag{8}$$

when the particle stays on the same site, and to

$$\begin{aligned} \langle\langle n'_j, m'|H_S + H_t - i\partial_t|n_{i\neq j}, m\rangle &= \int_0^T e^{i(m-m')\Omega t} J_{ij} \times \\ \exp\left(\frac{i}{\Omega}\left(A_j \sin(\Omega t + \phi_j) - A_i \sin(\Omega t + \phi_i)\right)\right)&, \end{aligned} \tag{9}$$

when the particle hops from site $i$ to site $j$. In eqs. (8) and (9), we label by $n_i$ the only non-zero occupation number of $\{n_i\}$. We can further use the Jacobi-Anger expansion to simplify eq. (9) to

$$\begin{aligned} &\langle\langle n'_j, m'|H_S + H_t - i\partial_t|n_{i\neq j}, m\rangle = \\ &- \mathcal{J}_{m'-m}\left(\rho_{ij}\right) e^{i(m'-m)\phi_{ij}} J_{ij}, \end{aligned} \tag{10}$$

with $\mathcal{J}_n(x)$ the $n$-th Bessel function of the first kind, and the definition

$$\rho_{ij} e^{i\phi_{ij}} = (A_j e^{i\phi_j} - A_i e^{i\phi_i})/\Omega. \tag{11}$$

### Perturbation theory

Some additional intuition can be found in writing the Floquet perturbation theory [3, 4] for the effective time-independent Hamiltonian $H_{\mathrm{eff}}$ that describes the time evolution for timescales greater than $T$, in the sense that

the time-evolution operator is

$$
\begin{aligned}
U(t+T,t) &= \exp\left(-i\int_t^{t+T}(H_S+H_t)\mathrm{d}t\right) \\
&= \exp\left(-iH_{\mathrm{eff}}T\right)
\end{aligned} \tag{12}
$$

For a Fourier-expanded time-periodic Hamiltonian,

$$
H(t) = \sum_m H_m e^{im\Omega t}, \tag{13}
$$

we can write a perturbation expansion for $H_{\mathrm{eff}}$ in orders of $1/\Omega$. Up to first order, this reads

$$
\begin{aligned}
H_{\mathrm{eff}} &= H_{0\Omega} + H_{1\Omega} + \mathcal{O}\left(\frac{1}{\Omega^2}\right) \\
&= H_{m=0} + \frac{1}{\Omega}\sum_{m=1}^{\infty}\frac{1}{m}[H_m, H_{-m}] + \mathcal{O}\left(\frac{1}{\Omega^2}\right).
\end{aligned} \tag{14}
$$

In our dynamically-modulated lattice, after the unitary transformation

$$
H' = U_t^\dagger[H_S + H_t - i\partial_t]U_t = \sum_i \omega_i a_i^\dagger a_i - \sum_m \sum_{ij} \mathcal{J}_m(\rho_{ij})\, e^{im(\Omega t+\phi_{ij})} J_{ij} a_i^\dagger a_j,
$$

with the definitions of $\mathcal{J}, \rho$, and $\phi$ as above, the Fourier components $H_m$ can be easily read out. The zero-th order of the perturbative expansion of eq. (14) is

$$
\begin{aligned}
H_{0\Omega} &= H_0 + H'_J = \sum_i \omega_i a_i^\dagger a_i - \sum_{ij} J'_{ij} a_i^\dagger a_j, \\
J'_{ij} &= J_{ij}\mathcal{J}_0(\rho_{ij}),
\end{aligned} \tag{15}
$$

i.e. similar to the starting $H_S$ of the static lattice, but with rescaled (but still real) couplings $J'_{ij}$. The first-order term is

$$
\begin{aligned}
H_{1\Omega} &= \sum_{m=1}^{\infty}\frac{(-1)^m}{\Omega m}\sum_{ijpq}\mathcal{J}_m(\rho_{ij})\mathcal{J}_m(\rho_{pq})J_{ij}J_{pq}e^{im(\phi_{ij}-\phi_{pq})} \\
&\quad\times [a_i^\dagger a_q \delta_{jp} - a_p^\dagger a_j \delta_{iq}] \\
&= \sum_{ij} 2i \sum_{m=1}^{\infty}\frac{(-1)^m}{\Omega m}\sum_p \mathcal{J}_m(\rho_{ip})\mathcal{J}_m(\rho_{pj})J_{ip}J_{pj} \\
&\quad\times \sin(m(\phi_{ip}-\phi_{pj}))a_i^\dagger a_j,
\end{aligned} \tag{16}
$$

The (purely imaginary) term after the first sum sign can obviously be interpreted as a new coupling amplitude, $J''_{ij}$, which is added to $J'_{ij}$, thus introducing a complex phase. The obvious interpretation of these terms is hopping from one site to another through one intermediate site. In the same way, terms of higher order in $1/\Omega$ represent hopping through an increasing number of intermediate sites.

**Honeycomb lattice**

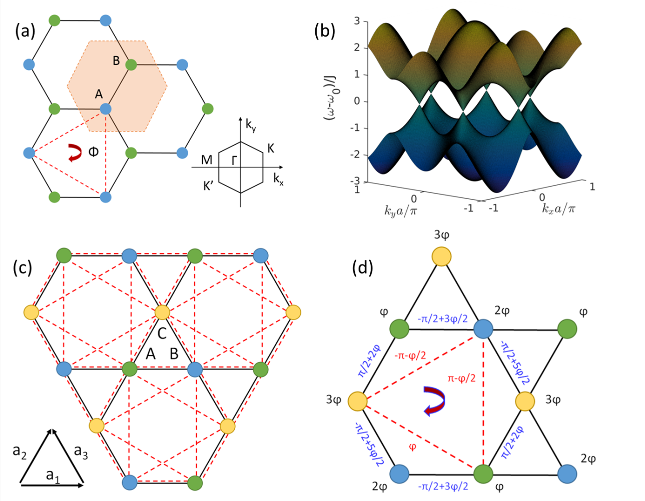


FIG. 1. (a): Honeycomb lattice with two sites A and B in the primitive cell (highlighted in orange). The Haldane model involves a complex second-neighbor hopping, which results in a magnetic flux enclosed in the red triangle. The Brillouin zone in reciprocal space is also shown. (b): Band structure of the lattice with first-neighbor coupling $J$ and zero flux $\Phi$. Six Dirac cones at the $K$-points are present. (c): Kagomé lattice, see also Fig. 1 in the main text. In the presence of the dynamic modulation, the zero-order terms of the perturbation-theory effective Hamiltonian are first-neighbor couplings (black lines), while the first-order terms are both first- and second-neighbor couplings (red dashed lines), induced by hopping through one intermediate site. (d): Definition of various phases under a modulation of constant amplitude, and phases (marked in black): $\varphi$ on site A, $2\varphi$ on site B, and $3\varphi$ on site C. In blue, the phase $\phi_{ij}$ as defined in eq. (11) is given for a clockwise hopping direction (indicated by the arrow in the center of the hexagon). With red, the phase $\phi_{ip} - \phi_{pj}$ entering eq. (16) is given, for the same hopping direction.

In the recent experimental observation of the Haldane model with cold atoms [4], the honeycomb lattice confining the atoms was 'shaken' by a periodic, elliptical modulation. In the reference frame of the lattice, this results in an inertial force on the atoms, which can be written as a site-dependent potential in the Hamiltonian. The strongest effect is obtained for circular modulation, in which case the Hamiltonian reads

$$
H_{lat} = \sum_{ij} t_{ij} c_i^\dagger c_j + \sum_i (C_i\cos(\Omega t) + S_i\sin(\Omega t)), \tag{17}
$$

with $t_{ij}$ the coupling constants, $c_i^\dagger, c_i$ the fermion creation and annihilation operators, $\Omega$ the frequency of the modulation, and $C_i, S_i$ – site-dependent constants. This can obviously also be implemented through a modulation of the form of eq. (2), with the remark that since both Hamiltonians are particle-number preserving, the particle statistics (bosons or fermions) are not important. Thus, all the considerations of Ref. [4] also hold for a lattice of optical resonators – and, in particular, a

Haldane model for photons on a honeycomb lattice can be implemented by choosing the $A_i$ and $\phi_i$ so as to match the $C_i$ and $S_i$ that can be read out of Ref. [4], i.e. setting

$$A_i \cos(\Omega t + \phi_i) = C_i \cos(\Omega t) + S_i \sin(\Omega t), \qquad \forall\, i. \quad (18)$$

However, we note that the circular 'shaking' implies an inertial force which is the same for all lattice sites, which, written in terms of a potential in the Hamiltonian, implies a spatial *gradient*. In other words, the $C_i$ and $S_i$ arising from this circular modulation in the cold-atom case are proportional to the position vector $\mathbf{r}_i$ of site $i$, which would then also be the case for $A_i$ when derived from eq. (18). Thus, replicating the cold atom system requires a gradient in the amplitude of the modulation of the frequency of the optical resonators, which is on one hand experimentally challenging, and on the other limits the scalability of such a system. Ideally, we would like to have a modulation which shares the spatial periodicity of the underlying lattice: this is, however, impossible in the case of the honeycomb lattice, for the following reason. This lattice has two sites in the unit cell (marked A and B in Fig. 1(a)). Assuming a modulation with the same periodicity, we are limited to two arbitrary amplitudes $A_A$ and $A_B$, and two arbitrary phases $\varphi_A$, $\varphi_B$. Whatever their values, however, looking at eq. (11), it is obvious that $\phi_{12} = \pi + \phi_{21}$, which means that $\phi_{12} - \phi_{21} = \pi$. Since all terms in the second-neighbor imaginary hoppings (eq. (16)) that come out of this modulation are proportional to $\sin(m(\phi_{12} - \phi_{21})$ with $m$ an integer, they are all zero.

In short, the Haldane model can be achieved in a dynamically modulated honeycomb lattice, but only through a spatially-varying amplitude of the modulation. This would limit the experimental feasibility of such a system, and in addition hampers the theoretical understanding through the Floquet band theory, since a modulation that breaks the spatial periodicity also makes it impossible to work in $k$-space. Fortunately, this problem can be easily overcome by choosing a slightly different geometry.

**Kagomé lattice**

The Kagomé lattice (illustrated in Fig. 1 here and Fig. 1(c) of the main text) has three lattice sites in the unit cell, which we label A, B, and C. With this lattice, it is possible to produce a non-zero Haldane-like flux, using a spatially periodic dynamic modulation. In fact, we can even impose a constant modulation amplitude $A_0$, and have spatial dependence only in the phase. As mentioned above, such a simple realization has the advantage of experimental scalability, and is also much easier to analyze theoretically, through two-dimensional Floquet band diagrams. To make matters simpler still, we set the phase of the modulation to $\varphi$, $2\varphi$, and $3\varphi$ on A, B, C, respectively, for some constant $\varphi$, which is the second free parameter of our system (together with $A_0$).

For the starting Hamiltonian, we assume a constant resonant frequency $\omega_0$ on all sites, and a constant first-neighbor coupling $J$ (along the black lines in Fig. 1(a)). In the presence of the modulation, the effective Hamiltonian of eq. (14) up to first order in perturbation theory can then be written in $k$-space as

$$\tilde{H} = \sum_{\mathbf{k}} \mathcal{A}_{\mathbf{k}}^\dagger \left(\omega_0 + \mathcal{H}(\mathbf{k})\right) \mathcal{A}_{\mathbf{k}} \quad (19)$$

with

$$\mathcal{A}_{\mathbf{k}}^\dagger = (a_{A,\mathbf{k}}^\dagger, a_{B,\mathbf{k}}^\dagger, a_{C,\mathbf{k}}^\dagger), \quad (20)$$

where $a_{A,\mathbf{k}}^\dagger$ is the Fourier transform of the $a_A^\dagger$ operator creating a particle on site $A$, and correspondingly for $B$ and $C$. The coupling matrix is given by

$$\mathcal{H}(\mathbf{k}) = -2J \begin{pmatrix} 0 & t_{AB}(\mathbf{k}) & t_{AC}(\mathbf{k}) \\ t_{AB}^*(\mathbf{k}) & 0 & t_{BC}(\mathbf{k}) \\ t_{AC}^*(\mathbf{k}) & t_{BC}^*(\mathbf{k}) & 0 \end{pmatrix}, \quad (21)$$

where the (dimensionless) couplings can be split into

$$\begin{aligned} t_{AB}(\mathbf{k}) &= (t_{AB,0} + t_{AB,1}) \cos(\mathbf{k}\mathbf{a}_1) + \\ &\quad t'_{AB,1} \cos(\mathbf{k}(\mathbf{a}_2 + \mathbf{a}_3)), \\ t_{AC}(\mathbf{k}) &= (t_{AC,0} + t_{AC,1}) \cos(\mathbf{k}\mathbf{a}_2) + \\ &\quad t'_{AC,1} \cos(\mathbf{k}(\mathbf{a}_1 - \mathbf{a}_3)), \\ t_{BC}(\mathbf{k}) &= (t_{BC,0} + t_{BC,1}) \cos(\mathbf{k}\mathbf{a}_2) + \\ &\quad t'_{BC,1} \cos(\mathbf{k}(\mathbf{a}_1 + \mathbf{a}_2)), \end{aligned} \quad (22)$$

where, in the first line, $t_{AB,0}$ is the first-neighbor coupling from site A to site B, $t_{AB,1}$ is the double-hop coupling (through site C) to a first-neighbor site B, and $t'_{AB,1}$ is the double-hop coupling (again through site C, but in a different direction) to a second-neighbor site B. The vectors $\mathbf{a}_i$ are defined such that $\mathbf{a}_1$ points from A to B, $\mathbf{a}_2$ points from A to C, and $\mathbf{a}_3$ points from B to C (see Fig. 1(a)). Simply put, the zero-th order effective Hamiltonian results in re-scaled first-neighbor couplings (black lines in Fig. 1(a)), while the first order results in all the couplings marked in dashed red lines in the Figure, which always involve an intermediate hopping, but are both first- and second-neighbor. The values of those couplings computed through (eq. (16)) are

$$
\begin{aligned}
t_{AC,0} = \mathcal{J}_0(2\rho_\varphi), \quad t_{AB,0} = t_{BC,0} = \mathcal{J}_0(\rho_\varphi) \\
t_{AB,1} = t'_{AB,1} = 2i\frac{J}{\Omega}\sum_m \frac{(-1)^m}{m}\mathcal{J}_m(\rho_{2\varphi})\mathcal{J}_m(\rho_\varphi)\sin(m(\varphi/2-\pi)) \\
t_{AC,1} = t'_{AC,1} = 2i\frac{J}{\Omega}\sum_m \frac{(-1)^m}{m}\mathcal{J}_m(\rho_\varphi)\mathcal{J}_m(\rho_\varphi)\sin(m\varphi) \\
t_{BC,1} = t'_{BC,1} = 2i\frac{J}{\Omega}\sum_m \frac{(-1)^m}{m}\mathcal{J}_m(\rho_{2\varphi})\mathcal{J}_m(\rho_\varphi)\sin(m(\pi+\varphi/2)),
\end{aligned} \tag{23}
$$

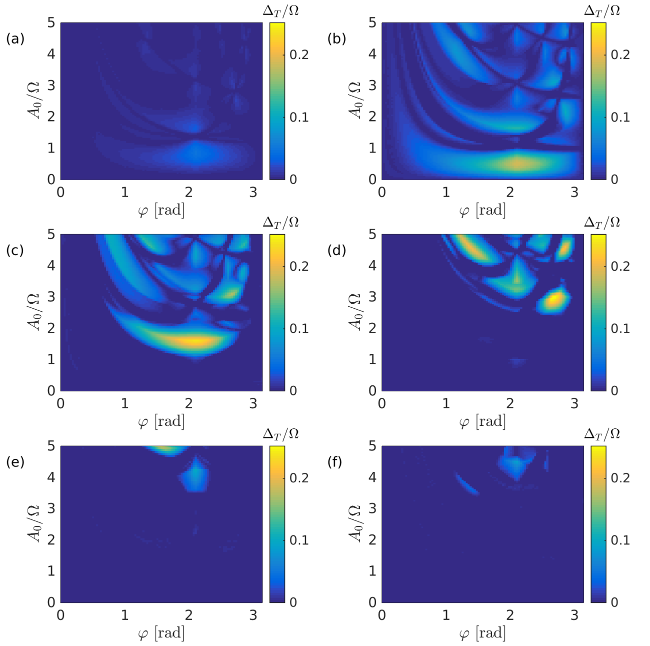


FIG. 2. The (largest) width of the opened band gap due to the dynamic modulation of frequency $\Omega$ vs. the amplitude $A_0$ and the phase angle $\varphi$ for the Kagomé lattice with first-neighbor coupling (a): $J = 0.1\Omega$; (b): $J = 0.3\Omega$; (c): $J = 0.5\Omega$; (d): $J = 0.7\Omega$; (e): $J = 0.9\Omega$; (f): $J = 1.1\Omega$. The colorbar scale is the same in all panels.

where $\rho_\varphi = 2(A_0/\Omega)|\sin(\varphi/2)|$ and $\rho_{2\varphi} = 2(A_0/\Omega)|\sin(\varphi)|$ are the amplitudes computed through eq. (16) for a phase difference between sites $i$ and $j$ of $\varphi$ and $2\varphi$, respectively. In Fig. 1(b), we illustrate the computation of the phases that enter the sine functions of eq. (23). Starting from the modulation phases (marked in black), one first computes the value of $\phi_{ij}$ (marked in blue) as defined in eq. (11) for all first neighbors, and then the values of $\phi_{ip} - \phi_{pj}$ (marked in red) that enter eq. (16).

## Numerical simulations

We note that this perturbation theory discussion is only used for a better intuitive understanding of the effect, but the topologically non-trivial bands are present even for values of $J$ that are comparable to $\Omega$. This is why in our work we mostly use the full diagonalization on the Floquet basis, i.e. we diagonalize the matrix of eq. (7). Numerically, we truncate the orders of $m\Omega$ by picking an $m_{\max}$ value and taking orders up to that, i.e. $|m|, |m'| \leq m_{\max}$. Convergence with respect to this parameter was always checked, and is reached very fast ($m_{\max} \approx 2$) for low values of $J$ when the different orders of the Floquet bands are well separated in frequency space. As $J$ becomes comparable to $\Omega$, higher orders are needed, but convergence was always reached at $m_{\max} = 10$, at most. The diagonalization of the effective static Hamiltonian of eq. (21) was only used for panels (b) of Fig. 2 and panels (a) and (c) of Fig. 3 of the main text. As is seen and can be expected, this matches the exact Floquet diagonalization very well for low $J/\Omega$, but becomes inadequate for higher values. Of course, that could in principle be fixed by higher orders in the perturbation expansion, but that would bring no further insight and is thus not really needed.

In Fig. 2 we show the width of the opened band gap $\Delta_T$ versus $A_0$ and $\varphi$, for $J$ from $0.1\Omega$ to $1.1\Omega$, computed by diagonalization on the Floquet basis. Panels (a) and (c) are shown in Fig. 3 of the main text (panels (b) and (d), respectively), but with a different scale of the colorbar. As $J$ increases, the amplitude $A_0$ needed to open a gap grows as well. This can at least qualitatively be understood through the following considerations. As $J$ becomes comparable to $\Omega$, Floquet bands of different orders $m$ start crossing, thus closing any potential band gaps. As $A_0$ increases, however, the rescaled first-neighbor coupling $J'_{ij}$ of eq. (15) generally decreases, since $\rho_{ij}$ is proportional to $A_0$, and the Bessel function $\mathcal{J}_0(x)$ has its maximum value at $x = 0$. Thus, the problem with mixing of bands of different orders can be avoided through a sufficiently large $A_0$.

* momchil.minkov@epfl.ch
[1] J. H. Shirley, Phys. Rev. **138**, B979 (1965).
[2] A. Eckardt, C. Weiss, and M. Holthaus, Physical Review Letters **95**, 1 (2005), arXiv:0601020 [cond-mat].
[3] H. Sambe, Phys. Rev. A **7**, 2203 (1973).
[4] G. Jotzu, M. Messer, R. Desbuquois, M. Lebrat, T. Uehlinger, D. Greif, and T. Esslinger, Nature **515**, 237240 (2014).
